# Supplementary material for: Interplay of capillary and Marangoni flows in micropillar evaporation
Source: arXiv:2202.05537 ancillary file (2022-03-23)
Supplement: Supplementary file 1 [file Supplementary_Material.pdf]

Supplementary Material for

# Interplay of capillary and Marangoni flows in micropillar evaporation

Göksel Yuncu[a,b], Yigit Akkus[a], Zafer Dursunkaya[b]

[a]ASELSAN Inc., 06200 Yenimahalle, Ankara, Turkey
[b]Middle East Technical University, 06800 Çankaya, Ankara, Turkey

A. Mesh Independence Study

B. Validation of the Meniscus Shape

C. Bi-directional Flow Model

D. Computational Scheme

E. Assessment of the Curvature Effect

# A. Mesh Independence Study

This section presents the mesh independence study for the meniscus shape, liquid transport, heat transport, and thermocapillary flow simulations at the cell-level model. While the mesh is being refined, the corresponding change in the selected parameter together with the corresponding solution time are reported in Fig. S1. The orange arrows on the plots indicate the chosen mesh for the model to obtain sufficiently accurate results with a low computational cost. Since the total number of degrees of freedom solved for (DOF= total number of nodes x dependent variables) depends on pillar dimensions, the equations solved in the problem, and the contact angle; simulations are conducted for relatively large pillar dimensions with a low contact angle $(d = 30\ \mu\text{m},\ l = 60\ \mu\text{m},\ h = 60\ \mu\text{m},\ \theta = 30°)$.

Properties of water at 25°C are utilized for mesh independence study. The periodic pressure difference is set to 15 Pa across a unit-cell during the flow modeling, and input heat flux is set to 60 W cm$^{-2}$. It should be noted that the corresponding Marangoni number is sufficiently high (*ca.* 250) to induce thermocapillary flow.

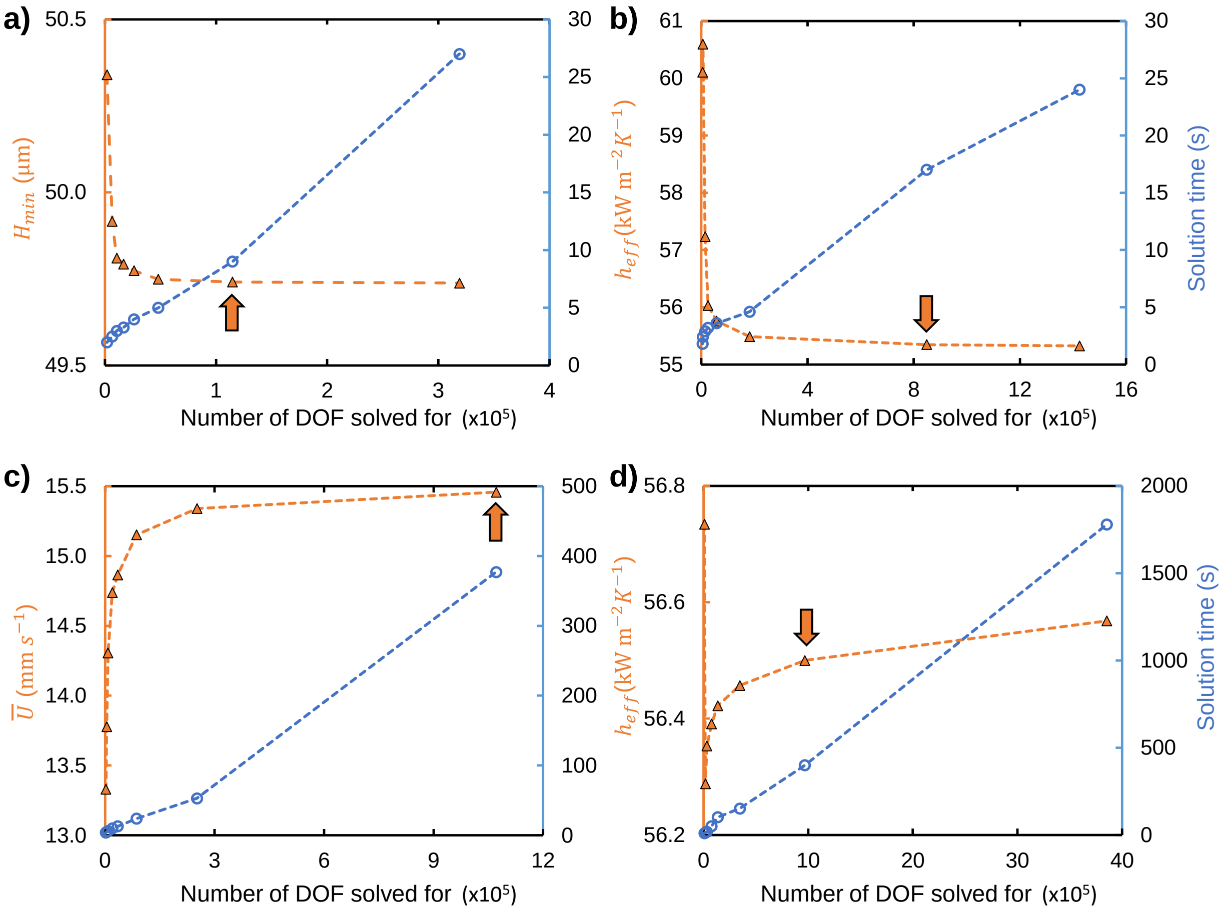


**Figure S1**: Mesh independence study at the cell-level **a)** meniscus shape, **b)** energy transport, **c)** liquid transport, and **d)** thermocapillary flow simulations. Minimum meniscus height, average velocity, and effective heat transfer coefficient are investigated across the solution time.

## B. Validation of the Meniscus Shape

In the Meniscus Shape model, height expression is obtained for the liquid-vapor interface by solving the Young-Laplace equation (assuming a fully-pinned three-phase contact line to the pillar top) for a pillar configuration and contact angle. The height expressions are utilized to form the three-dimensional deformed meniscus as a problem domain for remaining cell-level models. Although a sweep solution for various contact angles is conducted to capture the effect of the interface variation in the wicking direction, the accuracy of the entire model is very sensitive to the interface shape, especially near the pillar edge (contact line) where evaporation intensifies due to thinning film. The meniscus shape model is validated based on the laser interferometry measurements conducted by Adera *et al.* [1]. In the experiments, the vertical deformation in the lateral and diagonal directions was measured between adjacent cell centers, and several data were obtained along both directions.

In Fig. S2, height expressions obtained by solving the Y-L equation at several contact angles are compared with the experimentally measured vertical deformation data ($d = 5$ μm, $l = 12$ μm, $h =$ 82 μm). As shown in Fig. S2a, in the diagonal direction, vertical deformation prediction of the simulation for the pillar (receding) contact angle of θ=74° matches best with the experiment, whereas in the lateral direction, vertical deformation prediction of the simulation for the pillar (receding) contact angle of θ=66° matches best with the experiment. The average pillar contact angle can be calculated as 70° as considering the results in both directions. This value exactly matches with the average pillar contact angle prediction of Adera *et al.* [1].

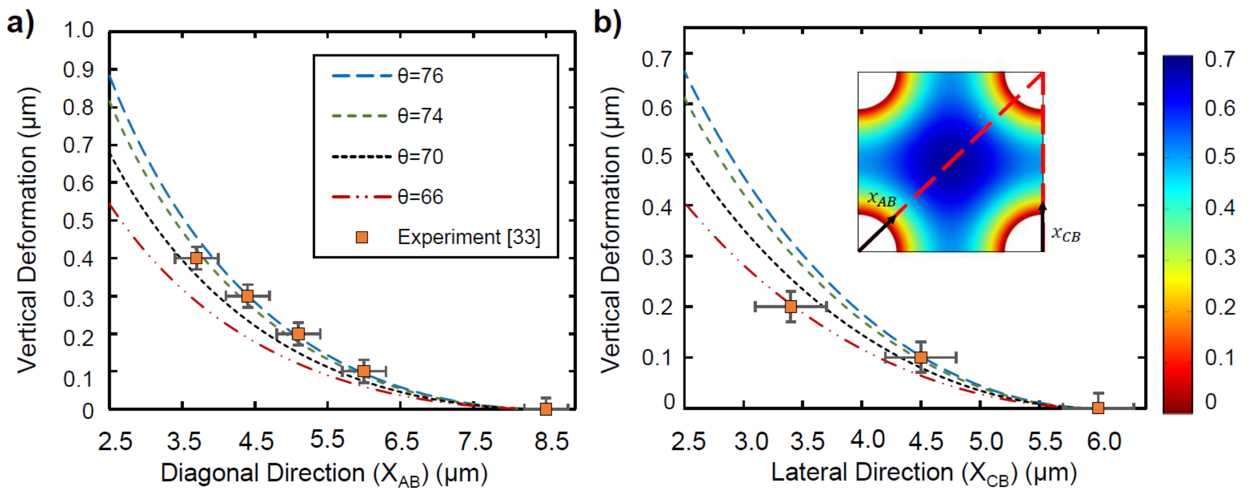


**Figure S2:** Comparison of vertical deformation prediction of the simulation and the experimental laser interferometry measurements [1]. Vertical deformation along the **a)** diagonal and **b)** lateral directions. The inset in Fig. S2b demonstrates vertical deformation contours on a meniscus with the contact angle of 70°.

## C. Bi-directional Flow Model

Since the square wick structure utilized in the experiments conducted by Adera *et al.* [1] is in contact with the liquid from all sides, the current model is adapted to solve the bi-directional flow in the device-level model. Due to the isotropic wicking flow in lateral directions, only one-quarter of the evaporator is considered as the problem domain. A two-dimensional domain is modeled to solve Darcy's law problem in COMSOL Multiphysics [2], and permeability values are acquired from the cell-level models as a function of geometry and capillary pressure.

Thin-film evaporation within the evaporator is modeled by the volumetric flow rate *via* point mass sources uniformly distributed over the domain. Applied heat flux is compensated by passive liquid propagation from the outer side of the domain. The capillary pressure is set to zero at two inlet boundaries, and the symmetric boundary condition is utilized at the remaining boundaries.

In Figure S3a, the problem domain is demonstrated with wicking directions and corresponding boundary conditions. Resultant capillary pressure and velocity magnitude variations on Device-1 are shown in Figures S3b and S3c.

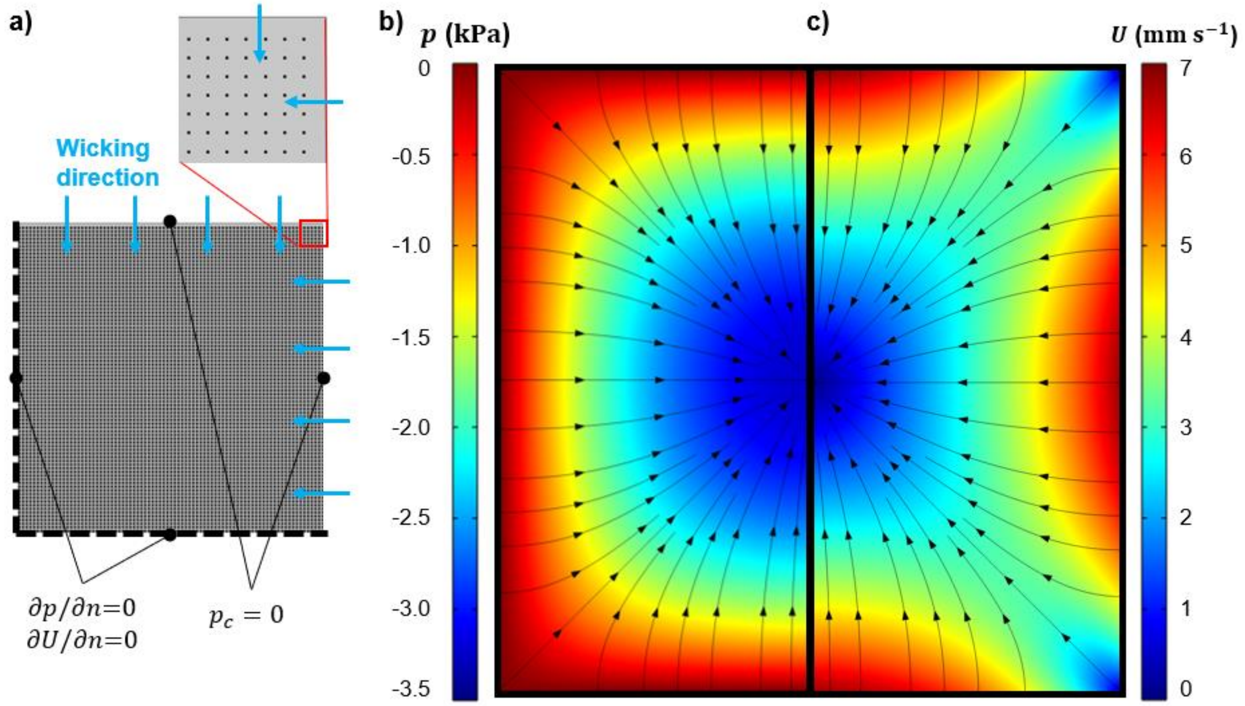


**Figure S3: a)** Problem domain of bi-directional flow model, and the boundary conditions. **b)** Capillary pressure variation with superimposed streamlines and **c)** velocity magnitude distribution with superimposed streamlines on Device-1. The applied heat flux is 40 W cm$^{-2}$ for the sample problem.

## D. Computational Scheme

In the model, numerous cell-level simulations are conducted at different contact angles and evaporative heat fluxes ($q_e''$) to create look-up tables for permeability ($\kappa$) and effective heat transfer coefficient ($h_{eff}$) that are employed in the device-level evaporator model. In addition to being functions of geometry and capillary pressure ($p_c$), permeability depends on the liquid temperature, while the effective heat transfer coefficient depends on the evaporative heat flux.

In the device-level, $q_{in}''(x)$ is applied at the bottom surface of the substrate with a thickness of $t_s$. The energy and liquid transport are coupled with the device-level flow and conduction models. Initially, the conduction in the substrate is neglected (*i.e.*, $q_{in}''(x) = q_e''(x)$ ), and the device-level flow model is solved to obtain $p_c$ distribution along the wicking direction by considering the conservation of mass, momentum, and energy. Since $h_{eff}$ is a function of $p_c(x)$, once having $p_c$ variation along the wicking direction in the fluid domain, the spatial distribution of $h_{eff}(p_c(x))$ is utilized in the conduction domain. Due to the presence of axial conduction through the substrate, a non-uniform effective heat transfer coefficient ($h_{eff}$), and non-uniform evaporation thereof, occurs along the wicking direction. Consequently, the evaporative heat flux ($q_e''(x)$) at each cell and average fluid temperature ($T_f$) is obtained in the conduction domain. Then $q_e''(x)$ and $T_f$ are utilized in the fluid domain to acquire $p_c$ distribution in the second and subsequent iterations. Thermal and flow domains are solved iteratively till the convergence of the dryout heat flux and evaporator superheat.

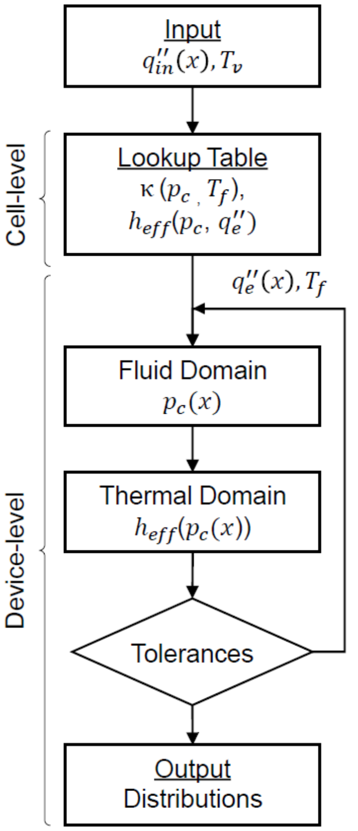


**Figure S4:** Computational scheme

## E. Assessment of the Curvature Effect

The effect of curvature on the evaporation is investigated at varying scales while keeping the aspect ratio ($d/h = 1.0$) and pitch-to-diameter ratios ($l/d = 1.8$) constant. The corresponding radius of curvature (RoC) values at a reference contact angle (θ=15°) are tabulated in Table S1. Since Wayner's approach includes the Kelvin effect (curvature effect) on the evaporation, the following equation is utilized to calculate the evaporation rate for the investigation [3]:

$$\dot{m}''_{evap} = a\,(T_{lv} - T_v) - b(p_c + p_d) \quad \text{(S1)}$$

$$a = \frac{2\hat{\sigma}}{2-\hat{\sigma}}\left(\frac{M}{2\pi R_u T_{lv}}\right)^{1/2}\left(\frac{M p_v h_{fg}}{R_u T_v T_{lv}}\right);\ b = \frac{2\hat{\sigma}}{2-\hat{\sigma}}\left(\frac{M}{2\pi R_u T_{lv}}\right)^{1/2}\left(\frac{p_v V_l}{R_u T_{lv}}\right) \quad \text{(S1a)}$$

where $T_v$, $T_{lv}$, $p_c$, $p_d$, $p_v$, $\hat{\sigma}$, $M$, $h_{fg}$, $R_u$, and $V_l$ are the vapor temperature, the temperature at the liquid-vapor interface, the capillary pressure, the disjoining pressure, the vapor pressure, mass accommodation coefficient, the molar mass of the liquid, the latent heat of vaporization, the universal gas constant, and specific volume of liquid, respectively. According to Equation S1, two factors determine the evaporation rate, the temperature difference (interfacial superheat) with a favorable effect and the capillary pressure (since disjoining pressure is negligible) with an adverse effect on the evaporation (as long as the interface is concave). The effective heat transfer coefficients are calculated by including ($h_{eff}$) and omitting ($h^*_{eff}$) the capillary pressure term to assess the curvature effect.

Effective heat transfer coefficient predictions are tabulated for varying capillary pressures, and the corresponding radius of curvatures (RoC) in Table S1. The effect of curvature becomes considerable only when the radius of curvature is a few microns or smaller. Considering the scale of the menisci in the past experimental studies modeled in the current work, the deviation between $h_{eff}$ and $h^*_{eff}$ is negligible, which verifies the fact that Kelvin effect can be negated in the problems of interest. Consequently, the utilization of the Schrage's relationships, which were derived based on the assumption of flat liquid-vapor interface [4], is justified.

**Table S1:** Effective heat transfer coefficients in the presence ($h_{eff}$) and omission ($h^*_{eff}$) of capillary pressure for the assessment of curvature effect on the evaporation.

| RoC | $p_c$ | $h_{eff}$ | $h^*_{eff}$ | Difference |
|---|---|---|---|---|
| μm | kPa | kW cm$^{-2}$ | kW cm$^{-2}$ | ‰ |
| 1.6 | -89.1 | 168.16 | 168.83 | 3.98 |
| 7.8 | -17.8 | 132.19 | 132.27 | 0.61 |
| 15.6 | -8.9 | 106.22 | 106.25 | 0.28 |
| 39.0 | -3.6 | 70.24 | 70.25 | 0.07 |
| 78.0 | -1.8 | 47.34 | 47.34 | 0.02 |

# References

[1] S. Adera, D. Antao, R. Raj, and E. N. Wang. Design of micropillar wicks for thin-film evaporation, Int. J. Heat Mass Tran., 101:280–294, 10 2016

[2] COMSOL Multiphysics® v. 5.6.www.comsol.com. COMSOL AB, Stockholm, Sweden.

[3] M. Sujanani and P.C. Wayner Jr. Microcomputer-enhanced optical investigation of transport processes with phase change in near-equilibrium thin liquid films. J. Coll. Interf. Sci 2:472—488, 1991.

[4] V. P. Carey. Liquid-vapor Phase Change Phenomena. Hemisphere Publishing House, New York, 1992.
